# Supplementary material for: Bounds and anomalies of inhomogeneous anomalous Hall effects
Source: arXiv:2408.15195 ancillary file (2025-02-14)
Supplement: Supplementary file 1 [file ahc_supp_sub.pdf]

# Supplemental Material for "Bounds and anomalies of inhomogeneous anomalous Hall effects"

Christopher Ard,[1] Evan Camrud,[2] Olivier Pinaud,[3] and Hua Chen[1,4]

[1]*Department of Physics, Colorado State University, Fort Collins, CO 80523, USA*
[2]*Department of Mathematics and Statistics, Middlebury College, Middlebury, VT 05753, USA*
[3]*Department of Mathematics, Colorado State University, Fort Collins, CO 80523, USA*
[4]*School of Materials Science and Engineering, Colorado State University, Fort Collins, CO 80523, USA*

## I. BOUNDS OF THE ANOMALOUS HALL CONDUCTIVITY IN A 2-PHASE COMPOSITE

We first consider a simple case. A 2D conductor has random magnetic domains with the following conductivity tensors

$$\boldsymbol{\sigma}_+ = \begin{pmatrix} \sigma_0 & -\sigma_\mathrm{h} \\ \sigma_\mathrm{h} & \sigma_0 \end{pmatrix}, \ \boldsymbol{\sigma}_- = \begin{pmatrix} \sigma_0 & \sigma_\mathrm{h} \\ -\sigma_\mathrm{h} & \sigma_0 \end{pmatrix}, \tag{1}$$

where $\sigma_0$ and $\sigma_h$ are positive constants. The spatial variation of the local conductivity tensor of the system is described by

$$\boldsymbol{\sigma}(\boldsymbol{r}) = h(\boldsymbol{r})\boldsymbol{\sigma}_+ + [1 - h(\boldsymbol{r})]\boldsymbol{\sigma}_-, \tag{2}$$

where $h(\boldsymbol{r}) = 1$ in the domains with the local conductivity tensor $\boldsymbol{\sigma}_+$, and 0 otherwise. We would like to understand the behavior of the effective conductivity tensor $\bar{\boldsymbol{\sigma}}$ defined as

$$\langle \boldsymbol{j} \rangle = \bar{\boldsymbol{\sigma}} \cdot \langle \boldsymbol{E} \rangle, \tag{3}$$

where $\langle \dots \rangle$ means spatial average. In general $\bar{\boldsymbol{\sigma}}$ depends on the form of $h(\boldsymbol{r})$. So we will focus on the bounds of the components of $\bar{\boldsymbol{\sigma}}$.

We first perform a duality transformation which can transform $\boldsymbol{\sigma}(\boldsymbol{r})$ to diagonal tensors. The general form of the duality transformation is [1]

$$\boldsymbol{\sigma}' = (a\boldsymbol{\sigma} + b\boldsymbol{R}_\perp) \cdot (c\boldsymbol{I} + d\boldsymbol{R} \cdot \boldsymbol{\sigma})^{-1}, \tag{4}$$

where

$$\boldsymbol{R}_\perp = \begin{pmatrix} 0 & -1 \\ 1 & 0 \end{pmatrix} \tag{5}$$

is the $\pi/2$ rotation matrix, and $a, b, c, d$ are arbitrary constants. It can be proved [1, 2] that the effective conductivity tensors for $\boldsymbol{\sigma}'$ and $\boldsymbol{\sigma}$ are related by the following equation

$$\bar{\boldsymbol{\sigma}}' = (a\bar{\boldsymbol{\sigma}} + b\boldsymbol{R}_\perp) \cdot (c\boldsymbol{I} + d\boldsymbol{R}_\perp \cdot \bar{\boldsymbol{\sigma}})^{-1}, \tag{6}$$

which will be used later to obtain the bounds of $\bar{\boldsymbol{\sigma}}$ from that of $\bar{\boldsymbol{\sigma}}'$.

$\boldsymbol{\sigma}'$ can be made diagonal by choosing $a = d = 1$ and

$$b = c = \sqrt{\sigma_0^2 + \sigma_h^2} \equiv \sqrt{\Delta}. \tag{7}$$

The explicit form of $\boldsymbol{\sigma}'$ in different domains, $\boldsymbol{\sigma}'_\pm$, is

$$\boldsymbol{\sigma}'_\pm = \frac{2\sigma_0\sqrt{\Delta}}{\sigma_0^2 + (\sqrt{\Delta} \mp \sigma_h)^2}\boldsymbol{I} \equiv \sigma'_\pm \boldsymbol{I}. \tag{8}$$

We have therefore transformed the original problem into a problem of finding the effective conductivity of the composite formed by two phases with different isotropic conductivities. The bounds of such an effective conductivity have been given in [3, 4], obtained using variational approaches. When applied to our problem they give

$$\bar{\sigma}' \in \left[\sigma'_- \frac{\sigma'_-\sigma_0 + (1+p)\sigma_h}{\sigma'_-\sigma_0 + (1-p)\sigma_h}, \sigma'_+ \frac{\sigma'_+\sigma_0 - (2-p)\sigma_h}{\sigma'_+\sigma_0 - p\sigma_h}\right], \tag{9}$$

where $p$ is the area ratio of domains with $\boldsymbol{\sigma}_+$. According to [4], the bounds are realized when the composite has the form of packed coated cylinders (in 2D). In our case, such a configuration means that the system can be partitioned into circular coated cells of arbitrary sizes with the core being one domain and the shell or coating being the other domain, and the area ratio of the two domains in each cell is fixed to $p/(1-p)$. Now let $\bar{\boldsymbol{\sigma}} \equiv \bar{\sigma}_0 \boldsymbol{I} + \bar{\sigma}_h \boldsymbol{R}_\perp$. Eq. (6) indicates that

$$\bar{\sigma}' = \frac{\bar{\sigma}_0}{\sqrt{\Delta} - \bar{\sigma}_h}, \quad (10)$$
$$\bar{\sigma}_0^2 + \bar{\sigma}_h^2 = \sigma_0^2 + \sigma_h^2 = \Delta,$$

from which we can obtain

$$\bar{\sigma}' = \frac{\sqrt{\Delta - \bar{\sigma}_h^2}}{\sqrt{\Delta} - \bar{\sigma}_h}. \quad (11)$$

Combining Eqs. (9) and (11), we finally obtain the bounds of $\bar{\sigma}_h$:

$$\bar{\sigma}_h \in \left[ -\sigma_h + \frac{2p\sigma_0^2\sigma_h}{\sigma_0^2 + (1-p)^2\sigma_h^2},\ \sigma_h - \frac{2(1-p)\sigma_0^2\sigma_h}{\sigma_0^2 + p^2\sigma_h^2} \right], \quad (12)$$

which takes the values of $\pm\sigma_h$ when $p = 1$ and $p = 0$, respectively, as expected. More importantly, one can see that the absolute value of $\bar{\sigma}_h$ can never exceed $\sigma_h$. The two bounds reduce to the trivial value $(2p-1)\sigma_h$ when $\sigma_h/\sigma_0 \to 0$, and $(2p-1)\sigma_h$ is also in-between the two bounds.

We next consider a slightly more complex case: the two domains have the following conductivity tensors

$$\boldsymbol{\sigma}_+ = \begin{pmatrix} \sigma_1 & -\sigma_\mathrm{h} \\ \sigma_\mathrm{h} & \sigma_1 \end{pmatrix},\ \boldsymbol{\sigma}_- = \begin{pmatrix} \sigma_2 & \sigma_\mathrm{h} \\ -\sigma_\mathrm{h} & \sigma_2 \end{pmatrix}, \quad (13)$$

with $\sigma_1 \neq \sigma_2$. Thus there is certain correlation between the longitudinal and Hall conductivities. For example, if $\sigma_1 > \sigma_2$, one can say that the positive magnetization domains have larger conductivity than the negative magnetization domains. Such situations could happen during a magnetization reversal, when the domains with negative magnetization first nucleate at the regions with lower conductivities or more defects, which is physically sensible. Note that the sense of positive and negative is reversed when considering the other half of the hysteresis curve during the magnetization reversal. Assume one starts from the uniform positive magnetization case with positive anomalous Hall conductivity, and slowly decreases the magnetic field. Negative magnetization domains will start to nucleate at regions with smaller longitudinal conductivity. However, when one starts from the uniform negative magnetization in the other half of the hysteresis curve, *positive* magnetization domains will first nucleate at regions with smaller longitudinal conductivity. Thus the values of $\sigma_h(\boldsymbol{r})$ can be either positive- or negative-correlated with the longitudinal conductivity, depending on the material and on which half of the hysteresis curve is under consideration.

By using the same approach in the above section, after some algebra one can obtain the following bounds for $\bar{\sigma}_h$:

$$\bar{\sigma}_h/\sigma_h \in \left[ -1 + \frac{8p\sigma_2^2}{[(1-p)\sigma_1 + (1+p)\sigma_2]^2 + 4(1-p)^2\sigma_h^2},\ 1 - \frac{8(1-p)\sigma_1^2}{[(2-p)\sigma_1 + p\sigma_2]^2 + 4p^2\sigma_h^2} \right]. \quad (14)$$

Apparently $|\bar{\sigma}_h| < \sigma_h$, so that the absolute value of the effective Hall conductivity cannot exceed that of the local Hall conductivity. Nonetheless, Eq. (14) suggests that it is possible for the lower bound to go above the simple average $2p-1$ when

$$\sigma_2^2 \geqslant \left( \frac{1-p}{2}\sigma_1 + \frac{1+p}{2}\sigma_2 \right)^2 + (1-p)^2\sigma_h^2, \quad (15)$$

which is easily satisfied when $\sigma_2 > \sigma_1$, and $\sigma_h \ll \sigma_1$. Conversely, the upper bound can be lower than the simple average when

$$\sigma_1^2 \geqslant \left( \frac{2-p}{2}\sigma_1 + \frac{p}{2}\sigma_2 \right)^2 + p^2\sigma_h^2, \quad (16)$$

which is easily satisfied when $\sigma_1 > \sigma_2$ and $\sigma_h \ll \sigma_2$.

Interestingly, Eqs. (15) and (16) may explain the following behavior in certain experiments: When plotting the anomalous Hall conductivity versus the total magnetization, sometimes there is also hysteresis, which suggests that

the effective anomalous Hall conductivity is not strictly proportional to the total magnetization throughout the magnetization reversal. Note that the total magnetization is nothing but $(2p-1)M_0$, where $M_0$ is the saturated magnetization. Since the designations of $\sigma_1$ and $\sigma_2$ are interchanged for the two halves of the hysteresis curve, it is indeed possible to have a hysteretic dependence between $\bar{\sigma}_h$ (bounded by Eq. (14)) and the total magnetization, when Eqs. (15) or (16) are satisfied. We should nonetheless note that the simple correlation in Eq. (13) does not apply throughout the hysteresis curve, as the regions with $\sigma_1$ and $\sigma_2$ are independent of magnetization. So this conclusion needs to be verified by more realistic numerical calculations.

## II. PROOF OF THEOREM 1

We recall that the microscopic conductivity reads $\boldsymbol{\sigma}(\boldsymbol{r}) = \boldsymbol{\sigma}_0(\boldsymbol{r}) + \sigma_{\rm h}(\boldsymbol{r})\mathbf{R}_\perp$, for $\boldsymbol{\sigma}_0(\boldsymbol{r})$ a positive definite diagonal matrix with entries $\sigma_{xx}$ and $\sigma_{yy}$, and $\mathbf{R}_\perp$ the $\pi/2$ rotation matrix. We denote by $\bar{\boldsymbol{\sigma}}$ the corresponding effective conductivity with effective Hall conductivity $\bar{\sigma}_{\rm h}$. The assumptions in the theorem ensure that the effective conductivity is well-defined and constant [5].

The main ingredient of the proof is a variational formula for the homogenized coefficients. Before getting to this, the standard theory of stochastic homogenization gives first the following expression for the effective conductivity, see [6]:

$$\bar{\boldsymbol{\sigma}} = \lim_{L\to\infty} \boldsymbol{\sigma}^L, \tag{17}$$

where the Hall conductivity of $\boldsymbol{\sigma}^L$ is

$$\sigma_{\rm h}^L = \frac{1}{L^2}\int_{\Omega_L} \big(\boldsymbol{\sigma}(\mathbf{r})\nabla(\phi_\xi(\mathbf{r}) + \xi\cdot\mathbf{r})\big)\cdot \xi_\perp d\mathbf{r}. \tag{18}$$

Above, $\Omega_L = [-L/2, L/2]\times[-L/2, L/2]$, $\xi = (1,0)^T$, $\xi_\perp = (0,1)^T$ ($T$ is for transposition), and for each $u \in \mathbb{R}^2$, $\phi_u$ is the unique (weak) solution to the corrector equation

$$\nabla\cdot\Big(\boldsymbol{\sigma}(\boldsymbol{r})\nabla(\phi_u(\mathbf{r}) + u\cdot\mathbf{r})\Big) = 0 \qquad \text{in } \Omega_L, \tag{19}$$

equipped with zero Dirichlet conditions at the boundary of $\Omega_L$. Similar expressions hold for the diagonal terms in $\boldsymbol{\sigma}^L$ but these will not be needed.

In (17), the limit holds for almost all (in the probabilistic sense) realizations of the random fields $\sigma_{xx}$, $\sigma_{yy}$ and $\sigma_{\rm h}$, and (18), (19) are defined for one of these realizations. Working with $\boldsymbol{\sigma}^L$ instead of $\bar{\boldsymbol{\sigma}}$ makes it possible to make use of the following variational characterization of the homogenized conductivity. Further, we denote by $\boldsymbol{\sigma}_s^L = (\boldsymbol{\sigma}^L + (\boldsymbol{\sigma}^L)^T)/2$ (resp. $\boldsymbol{\sigma}_s = (\boldsymbol{\sigma} + \boldsymbol{\sigma}^T)/2)$) the symmetric part of $\boldsymbol{\sigma}^L$ (resp. $\boldsymbol{\sigma}$) and by $\boldsymbol{\sigma}_a^L = (\boldsymbol{\sigma} - (\boldsymbol{\sigma}^L)^T)/2$ (resp. $\boldsymbol{\sigma}_a = (\boldsymbol{\sigma} - \boldsymbol{\sigma}^T)/2)$) its antisymmetric part. Since (18) is the expression of the effective coefficient in standard periodic homogenization, we have, according to [4], page 277, for $\xi_s$ and $\xi_a$ two arbitrary vectors in $\mathbb{R}^2$,

$$\begin{pmatrix}\xi_s\\ \xi_a\end{pmatrix}\cdot\begin{pmatrix}-\boldsymbol{\sigma}_s^L & -\boldsymbol{\sigma}_a^L\\ \boldsymbol{\sigma}_a^L & \boldsymbol{\sigma}_s^L\end{pmatrix}\begin{pmatrix}\xi_s\\ \xi_a\end{pmatrix} =$$

$$\max_{\substack{\nabla\times e_s(\mathbf{r}) = 0\\ <e_s>=\xi_s}} \ \min_{\substack{\nabla\times e_a(\mathbf{r}) = 0\\ <e_a>=\xi_a}} \left\langle \begin{pmatrix}e_s\\ e_a\end{pmatrix}\cdot\begin{pmatrix}-\boldsymbol{\sigma}_s(\mathbf{r}) & -\boldsymbol{\sigma}_a(\mathbf{r})\\ \boldsymbol{\sigma}_a(\mathbf{r}) & \boldsymbol{\sigma}_s(\mathbf{r})\end{pmatrix}\begin{pmatrix}e_s\\ e_a\end{pmatrix}\right\rangle$$

where $\langle f\rangle = \int_{\Omega_L} f(\mathbf{r})d\mathbf{r}/L^2$. The critical points solution to the saddle point problem are $\bar{e}_s = (\nabla\phi_\zeta + \nabla\phi'_{\zeta'})/2$ and $\bar{e}_a = (\nabla\phi_\zeta - \nabla\phi'_{\zeta'})/2$, where $\zeta = \xi_s + \xi_a$, $\zeta' = \xi_s - \xi_a$ and $\phi'_{\zeta'}$ solves (19) with $\boldsymbol{\sigma}$ replaced by $\boldsymbol{\sigma}^T$ and $u = \zeta'$.

With $\xi_s = (1,1)^T/2$, $\xi_a = (1,-1)^T/2$, and the fact that $\boldsymbol{\sigma}_a = \sigma_{\rm h}\mathbf{R}_\perp$ as well as $\boldsymbol{\sigma}_a^L = \sigma_{\rm h}^L\mathbf{R}_\perp$, direct algebra shows that

$$\sigma_{\rm h}^L = \min_{\substack{\nabla\times e_s(\mathbf{r}) = 0\\ <e_s>=\xi_s}} \ \max_{\substack{\nabla\times e_a(\mathbf{r}) = 0\\ <e_a>=\xi_a}} F_{\sigma_{\rm h}}(e_s, e_a) \tag{20}$$

where $F_{\sigma_{\rm h}}(e_s, e_a) = <e_s\cdot\boldsymbol{\sigma}_s e_s> - <e_a\cdot\boldsymbol{\sigma}_s e_a> + 2 <\sigma_{\rm h} e_s\cdot\mathbf{R}_\perp e_a>$. We now bound $\sigma_{\rm h}^L$ above and below. For this, since the assumption $-\sigma_M \le \sigma_{\rm h} \le \sigma_M$ holds, we have, independently of the sign of $e_s\cdot\mathbf{R}_\perp e_a$,

$$-\sigma_M(e_s\cdot\mathbf{R}_\perp e_a) \le \sigma_{\rm h}(e_s\cdot\mathbf{R}_\perp e_a) \le \sigma_M(e_s\cdot\mathbf{R}_\perp e_a).$$

As a consequence, we obtain from the definition of $F_{\sigma_{\rm h}}$ the inequality

$$F_{-\sigma_M}(e_s,e_a) \le F_{\sigma_{\rm h}}(e_s,e_a) \le F_{\sigma_M}(e_s,e_a),$$

which, according to the variational principle (20), implies that

$$\sigma^L_{{\rm h},-} \le \sigma^L_{\rm h} \le \sigma^L_{{\rm h},+}. \tag{21}$$

Above, $\sigma^L_{{\rm h},\pm}$ is the homogenized Hall coefficient associated with the microscopic conductivity $\boldsymbol{\sigma}_\pm(\boldsymbol{r}) = \boldsymbol{\sigma}_0(\boldsymbol{r}) \pm \sigma_M \mathbf{R}_\perp$. To conclude the proof, it suffices then to show that $\lim_{L\to\infty} \sigma^L_{{\rm h},\pm} = \pm\sigma_M$. This is done as follows. In the same way as (18), we have the following expression for $\sigma^L_{{\rm h},+}$:

$$\sigma^L_{{\rm h},+} = \frac{1}{L^2}\int_{\Omega_L} \big(\boldsymbol{\sigma}_+(\mathbf{r})\nabla(\phi^+_\xi(\mathbf{r}) + \xi\cdot\mathbf{r})\big)\cdot\xi_\perp d\mathbf{r} \tag{22}$$

for the $\xi$ and $\xi_\perp$ defined earlier. The function $\phi^+_\xi$ is the weak solutions to (19) with $\boldsymbol{\sigma}$ replaced by $\boldsymbol{\sigma}_+$. Since the off-diagonal entries of $\boldsymbol{\sigma}_+$ are equal to $\pm\sigma_M$ and are therefore constant, $\phi^+_\xi$ is actually solving (19) with $\boldsymbol{\sigma}$ replaced by $\boldsymbol{\sigma}_0$, that is

$$\nabla\cdot\Big(\boldsymbol{\sigma}_0(\boldsymbol{r})\nabla(\phi^+_\xi(\mathbf{r}) + \xi\cdot\mathbf{r})\Big) = 0 \qquad \text{in } \Omega_L, \tag{23}$$

equipped with Dirichlet boundary conditions at the boundary of $\Omega_L$. Multiplying (23) by $\xi_\perp\cdot\mathbf{r}$ and integrating by parts yields

$$L^{-2}\int_{\Omega_L} \big(\boldsymbol{\sigma}_0(\mathbf{r})\nabla(\phi^+_\xi(\mathbf{r}) + \xi\cdot\mathbf{r})\big)\cdot\xi_\perp d\mathbf{r} = L^{-2}\int_{\partial\Omega_L} \boldsymbol{n}\cdot(\sigma_0(\mathbf{r})\xi)(\xi_\perp\cdot\mathbf{r})dS,$$

where the right-hand-side corresponds to line integrals along the boundary $\partial\Omega_L$ of $\Omega_L$ and $\boldsymbol{n}$ is the outward unit normal to $\partial\Omega_L$. We denote the last term above by $T_L$. This allows us to rewrite $\sigma^L_{{\rm h},+}$ as

$$\begin{aligned}\sigma^L_{{\rm h},+} &= \frac{1}{L^2}\int_{\Omega_L} \big(\boldsymbol{\sigma}_0(\mathbf{r})\nabla(\phi^+_\xi(\mathbf{r}) + \xi\cdot\mathbf{r})\big)\cdot\xi_\perp d\mathbf{r} + \frac{\sigma_M}{L^2}\int_{\Omega_L} \big(\mathbf{R}_\perp\nabla(\phi^+_\xi(\mathbf{r}) + \xi\cdot\mathbf{r})\big)\cdot\xi_\perp d\mathbf{r} \\ &= T_L + \sigma_M + \frac{\sigma_M}{L^2}\int_{\Omega_L} \big(\mathbf{R}_\perp\nabla\phi^+_\xi(\mathbf{r})\big)\cdot\xi_\perp d\mathbf{r}.\end{aligned}$$

Above, we used that $(\mathbf{R}_\perp\xi)\cdot\xi_\perp = 1$. Besides, the last term is equal to zero since $\phi^+_\xi$ vanishes on $\partial\Omega_L$. We now show that $\lim_{L\to\infty} T_L = 0$, which is a consequence of Birkhoff ergodic theorem. Indeed, direct calculations show that

$$T_L = \frac{1}{L^2}\int_{-L/2}^{L/2} \delta\sigma_{xx}(y)ydy = \int_{-1/2}^{1/2} \delta\sigma_{xx}(Ly)ydy,$$

where $\delta\sigma_{xx}(y) = \sigma_{xx}|_{x=L/2} - \sigma_{xx}|_{x=-L/2}$ (we recall that $\mathbf{r} = (x,y)$). We now exploit the separation of scales between $\delta\sigma_{xx}(Ly)$ and the function $y$. Let $N_L$ be the integer part of $\sqrt{L}$. We break the interval $[-1/2, 1/2]$ into $N_L$ intervals of length $1/N_L$ centered at $y_k = -1/2 + 1/(2N_L) + (k-1)/N_L$, for $k = 1, \cdots, N_L$. We denote these intervals by $I_k$. Hence,

$$T_L = \sum_{k=1}^{N_L}\int_{I_k} \delta\sigma_{xx}(Ly)ydy.$$

On each $I_k$, the function $y$ varies slowly compared to $\delta\sigma_{xx}(Ly)$ for large $L$, and we can write

$$T_L = \sum_{k=1}^{N_L} y_k \int_{I_k} \delta\sigma_{xx}(Ly)dy + o(1),$$

where $o(1)$ is a term that goes to zero as $L\to\infty$. Since the random field $\delta\sigma_{xx}$ is stationary and ergodic, Birkhoff ergodic theorem implies that

$$\lim_{L\to\infty} N_L \int_{I_k} \delta\sigma_{xx}(Ly)dy = \mathbb{E}\{\delta\sigma_{xx}\}.$$

Note that $\mathbb{E}\{\delta\sigma_{xx}\}$ does not depend on position by stationarity of $\delta\sigma_{xx}$. This shows that

$$\begin{aligned} T_L &= N_L^{-1}\sum_{k=1}^{N_L} y_k N_L \int_{I_k} \delta\sigma_{xx}(Ly)dy + o(1) \\ &= \mathbb{E}\{\delta\sigma_{xx}\} N_L^{-1}\sum_{k=1}^{N_L} y_k + o(1) \\ &= \mathbb{E}\{\delta\sigma_{xx}\}\int_{-1/2}^{1/2} y dy + o(1). \end{aligned}$$

In the last line, we used the fact that $N_L^{-1}\sum_{k=1}^{N_L} y_k$ is a Riemann sum for the integral $\int_{-1/2}^{1/2} ydy$. Since $\sigma_{xx}$ is stationary, it follows that $\mathbb{E}\{\sigma_{xx}\}$ is independent of position and as a consequence $\mathbb{E}\{\delta\sigma_{xx}\} = 0$. Hence $\lim_{L\to\infty} T_L = 0$ and $\lim_{L\to\infty} \sigma^L_{\mathrm{h},+} = \sigma_M$. We prove in the same way that $\lim_{L\to\infty} \sigma^L_{\mathrm{h},-} = -\sigma_M$.

We are now in position to conclude. Since $\lim_{L\to\infty} \sigma^L_{\mathrm{h},\pm} = \pm\sigma_M$ and $\lim_{L\to\infty} \sigma^L_{\mathrm{h}} = \bar{\sigma}_{\mathrm{h}}$, it suffices to pass to the limit in (21) to obtain $-\sigma_M \le \bar{\sigma}_{\mathrm{h}} \le \sigma_M$. This ends the proof of Theorem 1.

## III. EXACT FORMULA OF $\langle\sigma_{\mathrm{h}}(\mathbf{r})\rangle$

In this section we give an exact formula for $\langle\sigma_{\mathrm{h}}(\mathbf{r})\rangle$ defined in Eq. (10) of the main text. We use the series expansion for the error function and the binomial theorem to obtain

$$\langle\sigma_{\mathrm{h}}(\mathbf{r})\rangle = \sigma_{\mathrm{h}}\frac{2}{\sqrt{\pi}}\sum_{n=0}^{\infty}\sum_{l=0}^{2n+1}\frac{(-2)^n(2n-1)!!}{l!(2n+1-l)!}\frac{(H-H_c)^l}{\epsilon_H^l}\langle(1+r_{\mathrm{h}}C)M^{2n+1-l}\rangle. \tag{24}$$

Using Wick's theorem one can explicitly calculate $\langle CM^{2n+1-l}\rangle$ (nonzero for even $l$ only) and $\langle M^{2n+1-l}\rangle$ (nonzero for odd $l$ only) as:

$$\begin{aligned} \langle CM^{2n+1-l}\rangle &= \langle CM^{2n-2k+1}\rangle = \mathcal{V}_{CM}\,(2n-2k+1)!! \\ \langle M^{2n+1-l}\rangle &= \langle M^{2n-2k}\rangle = (2n-2k-1)!! \end{aligned} \tag{25}$$

where we have used $\langle M^2\rangle = 1$. We therefore have

$$\langle\sigma_{\mathrm{h}}(\mathbf{r})\rangle = \sigma_{\mathrm{h}}\frac{2}{\sqrt{\pi}}\sum_{n=0}^{\infty}\sum_{k=0}^{n}\frac{(-1)^n 2^k(2n-1)!!}{(n-k)!}\left[\frac{(H-H_c)^{2k+1}}{\epsilon_H^{2k+1}(2k+1)!} + \frac{(H-H_c)^{2k}}{\epsilon_H^{2k}(2k)!}r_{\mathrm{h}}\mathcal{V}_{CM}\right]. \tag{26}$$

## IV. HOMOGENIZED HALL CONDUCTANCE IN THE PRESENCE OF DOMAIN WALLS

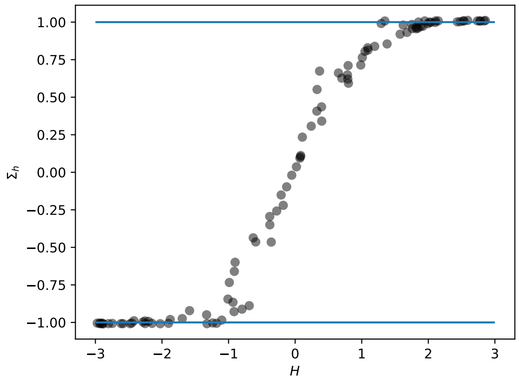


FIG. 1. Hall conductance $\Sigma_{\rm h}$ normalized to $\sigma_{\rm h}$, obtained by inverting the resistance tensor for random realizations of the domain configurations in the presence of domain wall resistivities. $\Sigma_{\rm h}/\sigma_{\rm h}$ is strictly bounded by $\pm 1$ within numerical error. The parameters used are $\xi \in [1\times10^{-3}, 5\times10^{-3}]$, $\sigma_\perp \in [-0.8, -0.1]$, $\sigma_\parallel \in [-0.7, -0.1]$ (with $|\sigma_\perp| > |\sigma_\parallel|$ enforced in all instances), $\sigma_{\rm h} \in [0.05, 0.5]$, $H_c = 0$, $\epsilon_W = 10$, $\sigma_0 = E_0 = \epsilon_H = 1$.

[1] G. W. Milton, Classical Hall effect in two-dimensional composites: A characterization of the set of realizable effective conductivity tensors, Phys. Rev. B **38**, 11296 (1988).
[2] A. M. Dykhne, Anomalous Plasma Resistance in a Strong Magnetic Field, Soviet Journal of Experimental and Theoretical Physics **32**, 348 (1971).
[3] Z. Hashin and S. Shtrikman, A Variational Approach to the Theory of the Effective Magnetic Permeability of Multiphase Materials, Journal of Applied Physics **33**, 3125 (1962).
[4] G. W. Milton, *The Theory of Composites*, Cambridge Monographs on Applied and Computational Mathematics (Cambridge University Press, 2002).
[5] L. Berlyand and V. Rybalko, *Getting acquainted with homogenization and multiscale*, Compact Textbooks in Mathematics (Birkhäuser/Springer, Cham, 2018).
[6] A. Bourgeat and A. Piatnitski, Approximations of effective coefficients in stochastic homogenization, Annales de l'Institut Henri Poincare (B) Probability and Statistics **40**, 153 (2004).
